# Supplementary material for: Syll: Open-Source Personal Automation with Cross-Surface Execution
Source: arXiv:2606.07594 source file (2026-05-28)
Supplement: Supplementary file 1 [file appendix.tex]

\section{Author Information}
\label{app:author_information}

We provide author contributions and contact information together in this appendix as follows:
\begin{itemize}
  \item \textbf{Borui Zhang}: Project leader of Syll; coordinated the overall research effort, guided the project direction, and contributed to code development.\\
  Contact: \texttt{zhang-br21@mails.tsinghua.edu.cn}
  \item \textbf{Bo Zhang}: Led the framework design, was primarily responsible for most of the system framework construction, and took the main role in code implementation and maintenance.\\
  Contact: \texttt{bo-zhang23@mails.tsinghua.edu.cn}
  \item \textbf{Chenghao Jiang}: Mainly designed the multimodal GUI grounding and localization tools and contributed to code development.\\
  Contact: \texttt{chenghao.jiang2022@outlook.com}
  \item \textbf{Minglei Shi}: Participated in project discussions, contributed constructive suggestions, and contributed to code and feature development.\\
  Contact: \texttt{sml25@mails.tsinghua.edu.cn}
  \item \textbf{Jie Zhou}: Provided overall guidance and supported the project with resources.\\
  Contact: \texttt{jzhou@tsinghua.edu.cn}
  \item \textbf{Jiwen Lu}: Corresponding author; provided overall guidance and supported the project with resources.\\
  Contact: \texttt{lujiwen@tsinghua.edu.cn}
\end{itemize}

\section{Additional Implementation Details}
\label{app:implementation}

The implementation is partitioned across \path{syll/agent/} for the core loop, context, skills, GUI planning, and tools; \path{syll/channels/} and \path{syll/bus/} for adapters and message flow; \path{syll/cron/} for scheduled routines; \path{syll/recorder/} for desktop recording; and \path{syll/web/} for FastAPI routes and the browser UI.

\section{Formal Model}
\label{app:formal_model}

\paragraph{Typed artifact-option process.}
We model Syll as a typed artifact-option process rather than a single reasoning-action transcript. The joint state contains both the external computer state and the agent-owned artifact state:
\[
  S_t = (X_t, A_t).
\]
A channel event is a partial observation of this state. Writing $\xi_t=(c_t,e_t)$ for the observed channel and raw event,
\[
  \xi_t \sim \Obsk(\cdot \mid S_t), \qquad
  m_t = \Adapt_{c_t}(e_t).
\]
The context builder then constructs a typed, task-relevant projection
\[
  C_t = \Phi(A_t,m_t) = (W_t,H_t,R_t,T_t,V_t,P_t).
\]
Because the true computer state is partially observable and the prompt is finite, $C_t$ is a lossy projection of the belief, not a sufficient statistic.
The policy first chooses an execution route and then emits a typed action:
\[
  r_t \sim \pi^R_\theta(\cdot \mid C_t), \qquad
  (\alpha_t,\hat{\psi}_t,\conf_t)
    \sim \pi^A_\theta(\cdot \mid C_t,r_t),
\]
with $a_t=(r_t,\alpha_t,\hat{\psi}_t,\conf_t)$. Here $\conf_t$ denotes the confirmation requirement emitted with the action, such as no gate, preview required, or explicit user approval; it is not a model confidence score and is retained as part of the audit record. Execution returns both an observation and an evidence artifact, after which the artifact state is updated:
\[
  (o_{t+1},z_{t+1}) = \Exec_{r_t}(\alpha_t,X_t), \qquad
  A_{t+1} = U_A(A_t,m_t,a_t,o_{t+1},z_{t+1},\hat{\psi}_t).
\]

\paragraph{Setup and observations.}
Let $X_t=(X_t^{\mathrm{os}},X_t^{\mathrm{app}},X_t^{\mathrm{web}}, X_t^{\mathrm{file}},X_t^{\mathrm{user}},G_t)$ be the partially observed computer state and let $A_t=(W_t,H_t,R_t,T_t,V_t,P_t,\Gamma_t)$ be the agent-owned artifact state. The joint state is $S_t=(X_t,A_t)$ and the observable history before the current decision is $h_t=(m_{1:t},a_{1:t-1},o_{1:t-1},z_{1:t-1})$, with belief $b_t(S)=\sP(S_t=S\mid h_t)$. Channel events are observations of this state:
\[
  \xi_t=(c_t,e_t)\sim\Obsk(\cdot\mid S_t), \qquad
  m_t=\Adapt_{c_t}(e_t).
\]

\paragraph{Process dynamics.}
The context builder is a lossy prompt projection, not a sufficient statistic:
\[
  \Phi:\mathcal{A}\times\mathcal{M}\to\mathcal{C},\qquad
  C_t=\Phi(A_t,m_t)=(W_t,H_t,R_t,T_t,V_t,P_t).
\]
The policy and executor decompose decisions into route choice, concrete action, expected postcondition, confirmation status, observation, and evidence:
\[
  r_t\sim\pi^R_\theta(\cdot\mid C_t),\qquad
  (\alpha_t,\hat{\psi}_t,\conf_t)\sim\pi^A_\theta(\cdot\mid C_t,r_t),
\]
\[
  (o_{t+1},z_{t+1})=\Exec_{r_t}(\alpha_t,X_t),\qquad
  A_{t+1}=U_A(A_t,m_t,a_t,o_{t+1},z_{t+1},\hat{\psi}_t).
\]

\paragraph{Skills as options.}
A full skill is $s=(\mu_s,\Omega_s,\pi_s,\beta_s,\Psi_s,\Gamma_s)$, an option with metadata, initiation predicate, intra-skill policy, derived termination, postconditions, and evidence schema. A demonstration induces
\[
  D_s=\{(I_i,\ell_i,\alpha_i,\psi_i,z_i)\}_{i=1}^{n}
\]
and terminates by
\[
  \beta_s(S_t)=\1[\Match(I_t,\Psi_s^{\mathrm{terminal}})],\qquad
  \Psi_s^{\mathrm{terminal}}=\mathit{meta}.\mathrm{success\_check}.
\]
Replay maintains $q_t(i)=\sP(p_t=i\mid\hat{\tau}_{\le t},D_s)$ with monotone kernel $\Pphase(i\mid j)$ that assigns $1-p_{\mathrm{adv}}$ to $i=j$, $p_{\mathrm{adv}}$ to $i=j+1$, and $0$ otherwise, retaining boundary mass at the terminal phase. The update and marginal policy are
\[
  q_t(i)\propto \Match(I_t,\psi_i)\sum_j\Pphase(i\mid j)q_{t-1}(j),
\]
\[
  \pi_s(a\mid C_t,D_s)=\sum_i q_t(i)\bigl[\lambda\delta_{\alpha_i}(a)
  +(1-\lambda)\pi_\theta(a\mid I_t,\ell_i,\psi_i)\bigr].
\]
\Cref{alg:demo_replay} is the MAP implementation: it stores only $p=\argmax_i q_t(i)$. Composition is admissible when $\Entails_A(\Psi_{s_1}^{\mathrm{terminal}},\Omega_{s_2})=1$.

\paragraph{ReAct as a degenerate case.}
The ReAct family interleaves free-form reasoning traces with environment actions \citep{yao2022react}; Reflexion and ReflAct add verbal feedback and goal-state reflection \citep{shinn2023reflexion,kim2025reflact}. It is recovered by taking a single channel, collapsing $A_t$ to a textual transcript $H_t$, removing persistent evidence artifacts and skills, and fixing the route to the environment:
\[
  (\tau_t,\alpha_t)\sim\pi_\theta(\cdot\mid H_t).
\]
Thus ReAct is the monolithic-text, no-option, no-audit special case.

\begin{algorithm}[H]
\footnotesize
\caption{Demonstration-conditioned replay (one episode).}
\label{alg:demo_replay}
\begin{algorithmic}[1]
\Require Skill
  $s = (\mathit{meta}, \mathit{traj}, \mathit{kf}, \mathit{trace})$
  with $N$ semantic steps; instruction $u$; context $C_t$; step budget $K$;
  wait interval $\delta$
\State $p \gets 0$;\quad evidence $E \gets \emptyset$
  \COMMENT{phase index, audit log}
\For{$k = 1$ to $K$}
  \State $I_k \gets \mathrm{CaptureScreenshot}()$;\quad
         $E \gets E \cup \{I_k\}$
  \If{$\mathrm{SuccessCheck}(I_k,\,
                            \mathit{meta}.\mathrm{success\_check})$}
    \State \Return $\langle \textsc{success},\, E \rangle$
  \EndIf
  \State $W \gets [\max(0, p{-}1),\, \min(N{-}1, p{+}1)]$
    \COMMENT{phase-positional window}
  \State $E_k \gets \{(\mathit{kf}[i],\, \mathit{trace}[i]) : i \in W\}$
    \COMMENT{Action ICL pack}
  \State $r \gets \mathrm{Actor}(C_t,\, u,\, E_k,\, p,\, I_k)$
    \COMMENT{$r.\mathrm{kind} \in
             \{\textsc{act}, \textsc{wait}, \textsc{recover}\}$}
  \If{$r.\mathrm{kind} = \textsc{wait}$}
    \State $\mathrm{Sleep}(\delta)$;\quad
           $E \gets E \cup \{r\}$;\quad \textbf{continue}
  \EndIf
  \If{$r.\mathrm{kind} = \textsc{recover}$}
    \State $E \gets E \cup \{r\}$;\quad \textbf{continue}
      \COMMENT{re-ground next iteration; $p$ unchanged}
  \EndIf
  \State $\mathrm{DesktopExecutor}(r.\mathrm{action})$;\quad
         $E \gets E \cup \{r.\mathrm{action}\}$
  \State $I_{k+1} \gets \mathrm{CaptureScreenshot}()$
  \If{$\Match(I_{k+1},\,
                      \mathit{trace}[p].\mathrm{expectation})$
       \textbf{ or } ($p{+}1 < N$ \textbf{ and }
        $\Match(I_{k+1},\,
                         \mathit{trace}[p{+}1].\mathrm{expectation})$)}
    \State $p \gets p + 1$
      \COMMENT{advance, possibly through a transient state}
  \EndIf
\EndFor
\State \Return $\langle \textsc{bounded\textnormal{-}failure},\, E \rangle$
\end{algorithmic}
\end{algorithm}

\subsection{Optimization with Auditability}
\label{app:formal_opt}

Auditability is modeled as a constraint rather than a reward bonus:
\[
  \max_\pi \E_\pi\!\left[\sum_{t=0}^{T}\gamma^t R(S_t,a_t)\right]
  \quad \mathrm{s.t.}\quad
  \E_\pi[\Covg(z_{1:T},\Psi)]\ge \kappa,
  \qquad a_t\in\mathcal{A}_{\mathrm{side}}\Rightarrow\conf_t=1.
\]
The Lagrangian form subtracts $\lambda(\kappa-\E[\Covg(z_{1:T},\Psi)])$, while the runtime enforces the constraint directly through confirmations, logs, screenshots, keyframes, and diffs.

\paragraph{Propositions and assumptions.}
\textbf{P1: Markov augmentation.} Given $P_X$, $\Obsk$, and $U_A$, the augmented process over $S_t=(X_t,A_t)$ is Markov before the current event is observed: $X_{t+1}$ depends on $X_t$ and $a_t$, while $A_{t+1}$ depends on $A_t$ and the current message, action, observation, evidence, and expected postcondition. \textbf{Assumption 1: artifact-summary ideal.} The artifact updater is designed to preserve history features needed for future action selection; in practice $C_t=\Phi(A_t,m_t)$ is lossy. Under this ideal, the standard belief-MDP reduction applies \citep{kaelbling1998planning}. \textbf{P2: demonstration as option.} $D_s$ induces an option with initiation predicate $\Omega_s$, intra-option policy $\pi_s$, and terminal-check termination $\beta_s$; therefore it is a semi-MDP action \citep{sutton1999between}. \textbf{P3: ReAct degeneracy.} Under the degenerate setting above, the typed artifact-option process reduces to ReAct because the only remaining decision is emitting a reasoning trace and an environment action from the textual transcript.

\section{Demonstration-Skill Schema}
\label{app:skill_schema}

Each demonstration skill referenced in the main paper is encapsulated as a self-contained directory whose fields parameterize the replay loop and the algorithmic episode in \Cref{alg:demo_replay}. The metadata holds the terminal success predicate that the verification step evaluates at the end of replay; the trajectory holds the deterministic-fallback event sequence dispatched by the executor; the keyframes anchor Action ICL retrieval at each step; and the trace gives per-step expectations used by the verification step as the phase index advances.

\begin{table}[tbp]
  \centering
  \caption{Demonstration-skill schema. Each field has a concrete replay role.}
  \label{tab:skill_schema}
  \begin{adjustbox}{width=\linewidth}
  \footnotesize
  
  \begin{tabular}{@{}>{\raggedright\arraybackslash}p{0.15\linewidth}
                    >{\raggedright\arraybackslash}p{0.44\linewidth}
                    >{\raggedright\arraybackslash}p{0.32\linewidth}@{}}
    \toprule
    \tblhead Field & Stored content & Replay and audit use \\
    \midrule
    \metric{$\mathit{meta}$}
      & Name, app context, aliases, preferred replay mode, terminal
        \texttt{success\_check} predicate
      & Registry summary; channel dispatch; terminal check in
        \Cref{alg:demo_replay} \\
    \metric{$\mathit{traj}$}
      & Ordered raw events: \texttt{click}, \texttt{type}, \texttt{key},
        \texttt{scroll}, \texttt{wait}, \texttt{hotkey}
      & Desktop executor input; deterministic fallback replay \\
    \metric{$\mathit{kf}$}
      & One screenshot per semantic step in the demonstration
      & Action ICL image anchor; human-readable audit evidence \\
    \metric{$\mathit{trace}$}
      & Per-step observation, intent, action, and a post-state
        expectation predicate
      & Phase indexing; actor prompt construction; per-step verification \\
    \bottomrule
  \end{tabular}
  \end{adjustbox}
\end{table}

\section{Companion Workspace Layout}
\label{app:workspace}

Syll stores its companion state as a directory of editable local artifacts. \Cref{tab:workspace_layout} enumerates the six artifact categories used by the persistent workspace update loop; the context builder resolves the relevant slices and injects them into $C_t$ during prompt construction, and both user edits and Syll's writes flow back into the same files.

\begin{table}[tbp]
  \centering
  \caption{Companion workspace layout. Each row is a directory of editable local
  artifacts that the context builder draws from when constructing $C_t$; the
  workspace update loop described in the main paper updates them
  through user edits and Syll's writes.}
  \label{tab:workspace_layout}
  \begin{adjustbox}{width=\linewidth}
  \footnotesize
  
  \begin{tabular}{@{}>{\raggedright\arraybackslash}p{0.18\linewidth}
                    >{\raggedright\arraybackslash}p{0.38\linewidth}
                    >{\raggedright\arraybackslash}p{0.34\linewidth}@{}}
    \toprule
    \tblhead Category & Representative files & Role \\
    \midrule
    Identity \& Rules
      & \texttt{IDENTITY.md}, \texttt{SOUL.md}, \texttt{AGENTS.md},
        \texttt{TOOLS.md}
      & Persona, operating constraints, behavioural rules, registered tools \\
    Profile \& Memory
      & \texttt{USER.md}, \texttt{memory/MEMORY.md}, \texttt{daily\_notes/}
      & User-specific facts and accumulating conversation memory \\
    Lore \& Rituals
      & \texttt{lore/fragments.md}, \texttt{lore/rituals.md}
      & Long-term relationship context and proactive behavioural rituals \\
    Skill Registry
      & \texttt{skills/}, \texttt{gui\_skills/}, \texttt{aloha\_skills/}
      & Text-based and demonstration-based reusable skills \\
    Traces \& Evidence
      & \texttt{event\_logs/}, \texttt{trajectory.json}, \texttt{keyframes/}
      & Per-run audit trail consumed by the verification step \\
    Schedules
      & \texttt{cron/jobs.json}
      & Time- or event-triggered routines \\
    \bottomrule
  \end{tabular}
  \end{adjustbox}
\end{table}

\section{Cross-Surface Runtime and Browser-Native Control}
\label{app:cross_surface_runtime}
\label{sec:cross_surface_runtime}

Cross-surface continuity begins at the runtime. Every user-facing surface enters the same local executor loop and shares the same workspace context, so the agent operates over a single ongoing state rather than a set of disjoint applications. Syll realizes this through a unified channel-bus-agent-tool architecture. Channel adapters normalize inputs from diverse sources (web consoles, CLIs, messaging apps, and scheduled jobs) into a standardized message format, and an in-process bus coordinates inbound messages, proactive triggers, and tool observations on behalf of the executor. Regardless of the origin surface, the executor loads the relevant session, constructs the context $C_{t}$, queries the model, dispatches validated tool calls, and appends the resulting observations and audit artifacts to the session history.

The browser-native control surface is integral to the system. Through the web UI, users can inspect and edit core artifacts, including model configurations, identity documents, skills, and activity logs. Unlike developer-oriented gateways such as OpenClaw \citep{openclaw2025}, Syll treats browser-based interaction as a first-class runtime surface that keeps the agent's internal state visible and editable for non-expert users. Beyond serving end users, this architecture is designed for research and community extension: the core executor loop is decoupled from peripheral interfaces, so channels, tools, and skills interact through standardized boundaries and plain-text persistence rather than tightly coupled code, letting researchers isolate components, integrate new capabilities, and fork the system for custom experiments.

\section{Limitations}
\label{sec:limitations}

Syll inherits the main limitations of current agent systems. GUI execution can fail because of visual grounding errors, high-DPI coordinate mismatch, hidden state, modal dialogs, permissions, network delays, or application updates. The demonstration loop can reduce repeated effort, but a single recording is not a guarantee of robust generalization across all UI variants.

The current artifact also has evaluation gaps. The public demos show plausible workflows, but the project still needs controlled quantitative results against strong baselines. Human-friendly auditability is a core claim, so it should be measured with user studies rather than inferred from design alone.

Finally, self-hosting gives users control but also shifts responsibility to local configuration. API keys, channel credentials, desktop permissions, filesystem access, and GUI automation privileges must be handled carefully. For safety, destructive file operations, external messaging, purchases, account changes, or other side effects should require explicit confirmation and clear logs.

\section{Reproducibility Statement}
\label{sec:reproducibility}

Syll is released as an open-source Python package and repository. The package, CLI, and import path are \texttt{syll}. The current codebase uses Python 3.11+ and includes FastAPI web routes, Typer CLI commands, LiteLLM model access, PyQt-based desktop companion support, channel adapters, GUI tools, recorder modules, and tests for web routes, tool validation, GUI planning, voice routes, cron behavior, and dashboard integration.

To reproduce the artifact-level setup:
\begin{itemize}
  \item install with \texttt{python -m pip install syll} or from source with \texttt{pip install -e ".[dev]"};
  \item run \texttt{syll onboard} to create the local configuration and workspace;
  \item configure the chat/planner/actor model endpoints and any channel credentials in the local config;
  \item run \texttt{syll wake} for the server and web UI, and optionally \texttt{syll ghost} for the desktop companion process;
  \item run \texttt{pytest} and \texttt{ruff check syll/} for implementation checks.
\end{itemize}

For future benchmark results, each reported run should include the model versions, provider endpoints, operating system, display resolution, selected screen, GUI actor mode, maximum steps, channel configuration, random seeds where applicable, and full execution traces with screenshots or videos sufficient to audit success and failure cases.
